# Supplementary material for: Classification of 4d N=2 gauge theories
Source: arXiv:1309.5160 ancillary file (2019-05-30)
Supplement: Supplementary file 1 [file enumerate-gauge-theories.pdf]

First we define functions turning data into diagrams.

```

In[1]:= vsh[{xc_, yc_}, {SU[n_], _}, {w_, h_}] := {LightYellow,
  Disk[{xc, yc}, .2], Inset[Style[Text[n], 14, Black, Bold], {xc, yc}]}];

In[2]:= vsh[{xc_, yc_}, {SO[n_], _}, {w_, h_}] :=
  {LightYellow, Disk[{xc, yc - .1}, .2, {0, Pi}],
  Inset[Style[Text[n], 14, Black, Bold], {xc, yc}]}];

In[3]:= vsh[{xc_, yc_}, {USp[n_], _}, {w_, h_}] :=
  {LightYellow, Disk[{xc, yc + .1}, .2, {Pi, 2 Pi}],
  Inset[Style[Text[n], 14, Black, Bold], {xc, yc}]}];

In[4]:= vsh[{xc_, yc_}, {G2, _}, {w_, h_}] := {LightRed,
  Disk[{xc, yc + .1}, .2], Inset[Style[Text[G2], 14, Black, Bold], {xc, yc}]}];

In[5]:= vsh[{xc_, yc_}, {Matter, _}, {w_, h_}] := {LightGray, Disk[{xc, yc}, .1]}

In[6]:= graphlabel[bif[_], _] := ""

In[7]:= graphlabel[biff[_], _] := "/"

In[8]:= graphlabel[spinbif[_], _] := "S"

In[9]:= graphlabel[f[_], _] := f

In[10]:= ShowQuiver[x_] :=
  Module[{q = AsQuiver[x, 1]}, Graph[q[[1]], q[[2]], VertexShapeFunction -> vsh,
    GraphLayout -> "LayeredDigraphDrawing", DirectedEdges -> True]]

In[11]:= AsQuiver[{x_, {}}, n_] := {{{x, n}}, {}

In[12]:= AsQuiver[{x_, xs_}, n_] :=
  Module[{leaves = Table[AsQuiver[xs[[i, 2]], 10 n + i], {i, 1, Length[xs]}],
    edges, vertices},
  vertices = Flatten[({#[[1]]} & /@ leaves, 1];
  edges = Flatten[({#[[2]]} & /@ leaves, 1];
  {
    {{x, n}} ~Join~ vertices,
    Table[Labeled[{x, n} ⌀ {xs[[i, 2, 1]], 10 n + i}, graphlabel[xs[[i, 1]]],
      {i, 1, Length[xs]}] ~Join~ edges
  }]

```

This function obtains all the subsets of {i,j, ...} such that func[i]+func[j]+ ... ≤ max. Usually it doesn't return {i} if {i,j} is also allowed. To get really all the subsets, Use MaxOnly → False.

```

In[13]:= subsets[x_, func_, max_, h_, opts : OptionsPattern[]] := If[max < 0, {},
  Flatten[Table[
    Module[{next = Prepend[#, x[[i]]] & /@ subsets[x, func, max - func[x[[i]]], i]},
    If[OptionValue[MaxOnly] == True,
      If[next == {}, If[func[x[[i]]] ≤ max, {{x[[i]]}, {}}, next],
      If[func[x[[i]]] ≤ max, {{x[[i]]}, {} } ~Join~ next]], {i, h, Length[x]}]
  , 1]]

In[14]:= Options[branches] = {MaxOnly -> True, LevelOneOnly -> False};

In[15]:= Options[subsets] = {MaxOnly -> True, LevelOneOnly -> False};

```

This function lists all branches starting with gauge group “start”, with the

hyper's contribution to the beta function < "maxh". The matter contents allowed are specified by "choices". Usually returns only the maximal quiver, where no gauge groups or matters can be added. If you really want to get all, use MaxOnly → False.

Another options: LevelOneOnly→True returns only branches with length 2.

```
In[16]:= flip[bif[x_, y_]] := bif[y, x]

In[17]:= biff[bif[x_, y_]] := biff[y, x]

In[18]:= flip[spinbif[x_, y_]] := spinbif[y, x]

In[19]:= branches[start_, maxh_, choices_, opts : OptionsPattern[]] :=
  Module[{next, nextbranches, leaves},
    next =
      Select[
        Flatten[If[MatchQ[start, #[[1]], start /. #, {}] & /@ choices],
          contrib[#] ≤ maxh &
        ];
    nextbranches = Sort[Flatten[
      If[#[[2]] === Matter || OptionValue[LevelOneOnly],
        {{#, {#[[2]], {}}}},
        Module[{gauge = #[[2]]},
          Function[x, {#, x}] /@
            branches[gauge, 2 hvee[gauge] - contrib[flip[#]], choices, opts]]] &
        /@ next
      , 1], contrib[#1[[1]]] < contrib[#2[[1]]] &];
    leaves = subsets[nextbranches, contrib[#[[1]]] &, maxh, 1, opts];
    If[OptionValue[MaxOnly] == True,
      If[leaves == {}, {{start, {}}, ({start, #} & /@ leaves)},
        {{start, {}}}~Join~ ({start, #} & /@ leaves)]]
```

Another way to remove clutter: RemoveVeryObvious[...] removes theories made of just one branch or two small branches.

```
In[20]:= RemoveVeryObvious[x_] := Select[x, (Length[#[[2]]] > 2 || (Length[#[[2]]] == 2 &&
  (contrib[#[[2], 1, 1]] - hvee[#[[1]]]) (contrib[#[[2], 2, 1]] - hvee[#[[1]]]) < 0)) &]
```

You can also check the structure of the branches. depth[..] gives the overall depth, and lengths[..] gives the list of the lengths of individual branches.

```
In[21]:= depth[{Matter, {}}] := 0

In[22]:= lengths[{Matter, {}}] := {0}

In[23]:= depth[{_, {}}] := 1

In[24]:= lengths[{_, {}}] := {1}

In[25]:= lengths[{_, xs_}] := (1 + depth[#[[2]]) & /@ xs

In[26]:= depth[x_] := Max[lengths[x]]

In[27]:= CartanMatrix[x_] := Module[{a, b}, a = AdjacencyMatrix[x];
  b = -a - Transpose[a]; Do[b[[i, i]] = 2, {i, 1, Length[a]}]; b]

In[28]:= DynkinQ[x_] := And@@ ((# ≥ 0) & /@ N[Eigenvalues[CartanMatrix[x]]])
```

```
In[29]:= NonDynkinQ[x_] := ! DynkinQ[x]
```

Here come the data. First, the dual Coxeter.

```
In[30]:= hvee[Matter] := -1
```

```
In[31]:= hvee[SU[n_]] := n
```

```
In[32]:= hvee[SO[n_]] := n - 2
```

```
In[33]:= hvee[USp[n_]] := n / 2 + 1
```

```
In[34]:= hvee[G2] := 4
```

Possible matters are categorized into a few cases. Each is a list of containing gauge  $\rightarrow$  {list of matters}

```
In[35]:= bifunds = {SU[n_] => Table[bif[SU[n], SU[m]], {m, Max[Ceiling[n/2], 2], n-1}],
    SO[n_] => Table[bif[SO[n], USp[m]],
        {m, Max[2 Ceiling[n/4] - 2, 2], 2 Floor[n/2] - 2, 2}],
    USp[n_] => Table[bif[USp[n], SO[m]], {m, Max[n/2 + 2, 3], n+1}]
};
```

```
In[36]:= rarebifunds = {
    USp[n_] => Table[bif[USp[n], USp[m]], {m, Max[n-2, 2], n}],
    USp[n_] => Table[bif[USp[n], SU[m]], {m, Max[n/2, 3], n}],
    SO[n_] => Table[bif[SO[n], SU[m]], {m, Max[n/2, 2], n-2}],
    SO[7] => Table[spinbif[SO[7], USp[m]], {m, 2, 10, 2}],
    USp[n_? (# <= 10 &)] => {spinbif[USp[n], SO[7]]},
    SU[n_? ((EvenQ[#] && # >= 5) &)] => {bif[SU[n], USp[n-2]]},
    G2 => Table[bif[G2, USp[m]], {m, 2, 8, 2}],
    USp[n_? (# <= 8 &)] => {bif[USp[n], G2]}
};
```

```
In[37]:= idents = {
    SU[4] => {biff[SO[6], USp[2]], biff[SO[6], USp[4]]},
    SO[6] => {biff[SU[4], SU[2]], biff[SU[4], SU[3]]},
    SO[5] => {biff[USp[4], SO[4]], biff[USp[4], SO[5]], biff[USp[4], SO[6]]},
    USp[4] => {biff[SO[5], USp[2]]}
};
```

Due to my sloppy programming, the fields charged under one gauge group need to be given as a bifundamental with a second “imaginary” group called “Matter”.

```
In[38]:= matters = {
    SU[n_? ((# > 3) &)] => {asym[SU[n], Matter]},
    SU[6] => {asym3[SU[6], Matter]},
    USp[6] => {asym3[USp[6], Matter]},
    SO[n_? (# >= 9 && # <= 13 &)] => {spinor[SO[n], Matter]}
};
```

Now we define the beta function contributions.

```
In[39]:= contrib[bif[SU[n_], SU[m_]]] := m
```

```
In[40]:= contrib[bif[SU[n_], SO[m_]]] := m
```

```

In[41]:= contrib[bif[SU[n_], USp[m_]]] := m
In[42]:= contrib[bif[SO[n_], SU[m_]]] := 2 m
In[43]:= contrib[bif[SO[n_], SO[m_]]] := 2 m
In[44]:= contrib[bif[SO[n_], USp[m_]]] := m
In[45]:= contrib[bif[USp[n_], SU[m_]]] := m
In[46]:= contrib[bif[USp[n_], SO[m_]]] := m / 2
In[47]:= contrib[bif[USp[n_], USp[m_]]] := m
In[48]:= contrib[bif[USp[_], G2]] := 7 / 2
In[49]:= contrib[bif[G2, USp[m_]]] := m
In[50]:= contrib[spinbif[USp[_], SO[7]]] := 4
In[51]:= contrib[spinbif[SO[7], USp[m_]]] := m
In[52]:= contrib[asym[SU[n_], Matter]] := n - 2
In[53]:= contrib[asym3[SU[6], Matter]] := 3
In[54]:= contrib[asym3[USp[6], Matter]] := 5 / 2
In[55]:= contrib[spinor[SO[n_? (# ≥ 9 && # ≤ 12 &)], Matter]] := 4
In[56]:= contrib[spinor[SO[13], Matter]] := 8
In[57]:= contrib[biff[a_, b_]] := contrib[bif[a, b]]

```

This concludes the program. Let us explain the usage.

**branches[group, max, type]** gives all the combinations of branches starting with the specified “group”, with total one-loop contribution at most “max”, using hypers listed in “type”. For example,

```

In[58]:= branches[SU[6], 6, bifunds]
Out[58]= {{SU[6], {{bif[SU[6], SU[3]], {SU[3], {}}, {bif[SU[6], SU[3]], {SU[3], {}}}}},
  {SU[6], {{bif[SU[6], SU[4]], {SU[4], {{bif[SU[4], SU[2]], {SU[2], {}}}} }}},
  {SU[6], {{bif[SU[6], SU[5]], {SU[5],
    {{bif[SU[5], SU[4]], {SU[4], {{bif[SU[4], SU[2]], {SU[2], {}}}} }} }}},
  {SU[6], {{bif[SU[6], SU[5]], {SU[5], {{bif[SU[5], SU[4]], {SU[4], {{bif[SU[4],
    SU[3]], {SU[3], {{bif[SU[3], SU[2]], {SU[2], {}}}} }} }} }}},
  {SU[6], {{bif[SU[6], SU[5]], {SU[5], {{bif[SU[5], SU[3]], {SU[3], {}}}} }} }}

```

which is the list of raw data. To view graphically, use `ShowQuiver /@` :

```
In[59]:= ShowQuiver /@ branches[SU[6], 6, bifunds]
```

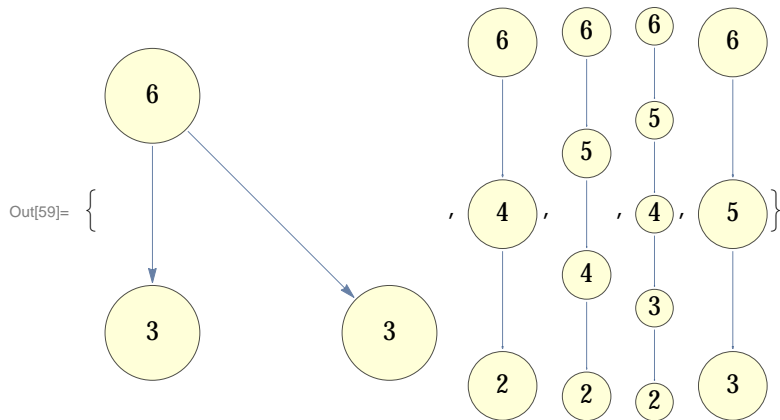

```
In[60]:= depth /@ branches[SU[6], 6, bifunds]
```

```
Out[60]= {2, 3, 4, 5, 3}
```

```
In[61]:= lengths /@ branches[SU[6], 6, bifunds]
```

```
Out[61]= {{2, 2}, {3}, {4}, {5}, {3}}
```

If you want to show non-maximal ones,

```
In[62]:= ShowQuiver /@ branches[SU[6], 6, bifunds, MaxOnly -> False]
```

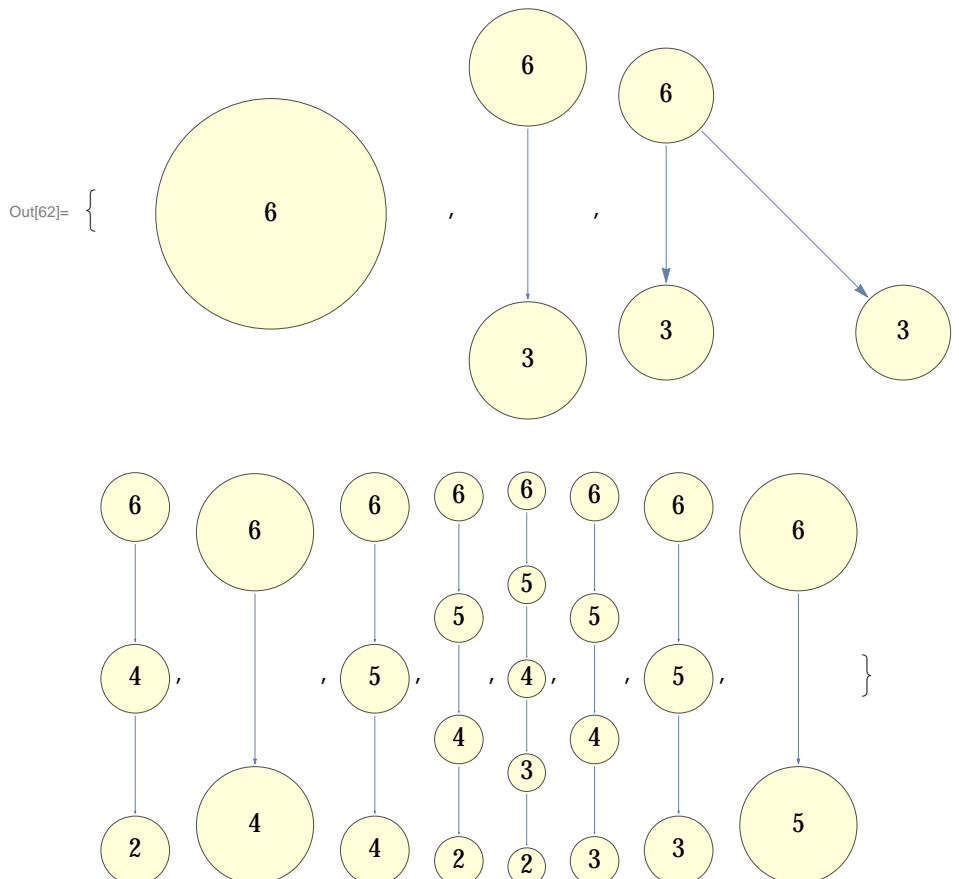

“bifunds” only contains SU-SU and SO-USp bifundamentals. If you want to use other matter fields coupled to just one simple factor, you should do

```
In[63]:= ShowQuiver /@branches[SU[6], 6, Join[bifunds, matters]]
```

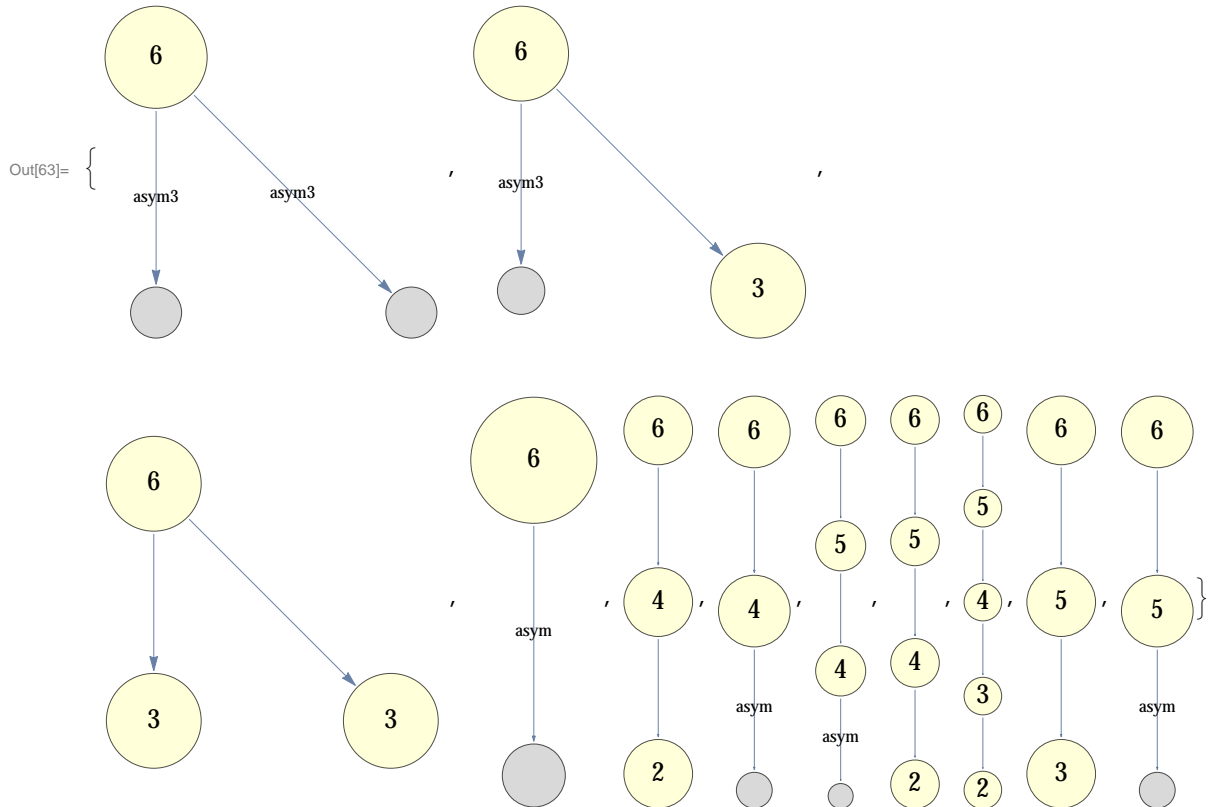

```
In[64]:= lengths /@branches[SU[6], 6, Join[bifunds, matters]]
```

```
Out[64]= {{1, 1}, {1, 2}, {2, 2}, {1}, {3}, {2}, {3}, {4}, {5}, {3}, {2}}
```

Gray circles are dummy targets which seem necessary to have an edge inside a Mathematica graph ...

SU-USp fundamentals etc. are included by doing

```
In[65]:= ShowQuiver /@branches[SU[6], 6, Join[bifunds, rarebifunds]]
```

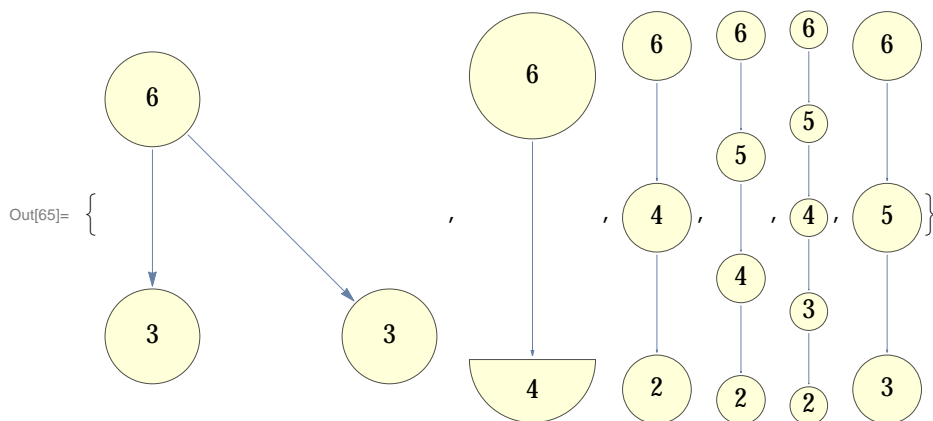

**SU(4)=SO(6) etc. can be taken into account by doing**

```
In[66]:= ShowQuiver /@ branches[SO[6], hvee[SO[6]], Join[bifunds, idents]]
```

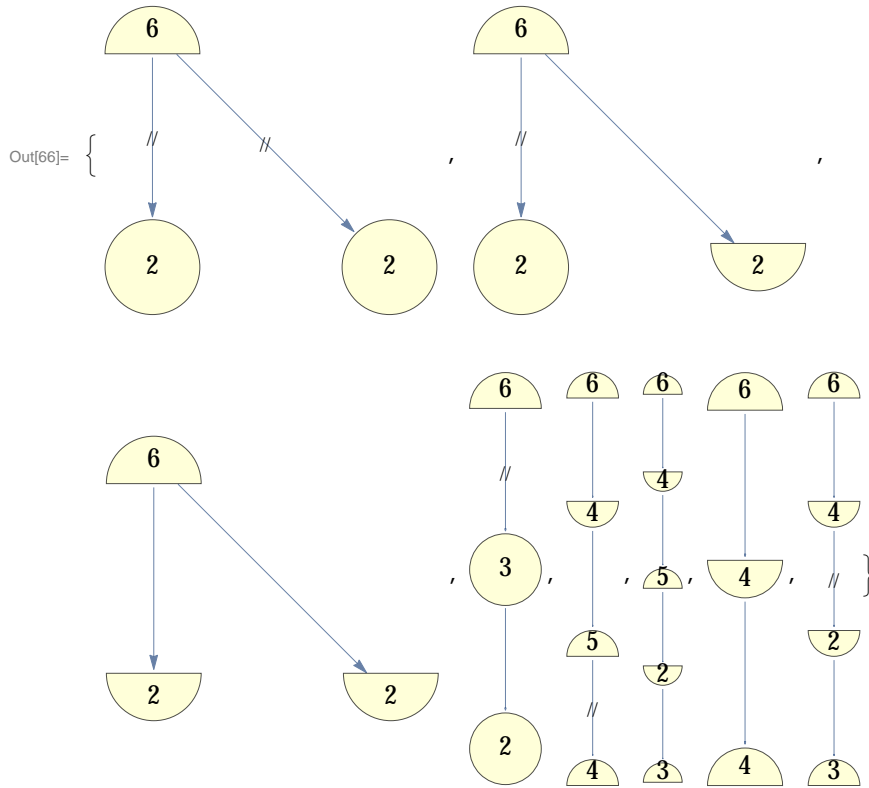

An edge marked with // signifies that the node closer to the trunk should be replaced according to the following rule:  $SU(4) \leftrightarrow SO(6)$ ,  $SO(5) \leftrightarrow USp(4)$ .

Summarizing: “bifunds” for standard SU-SU and SO-USp bifundamentals; “rarebifunds” for other bifundamentals, “matters” for other representations coupled to simple factors, and “idents” for the above identifications.

To remove rather obvious ones with just one branch or two small branches, do this

```
In[67]:= ShowQuiver /@ RemoveVeryObvious[branches[SU[6], 12, bifunds]]
```



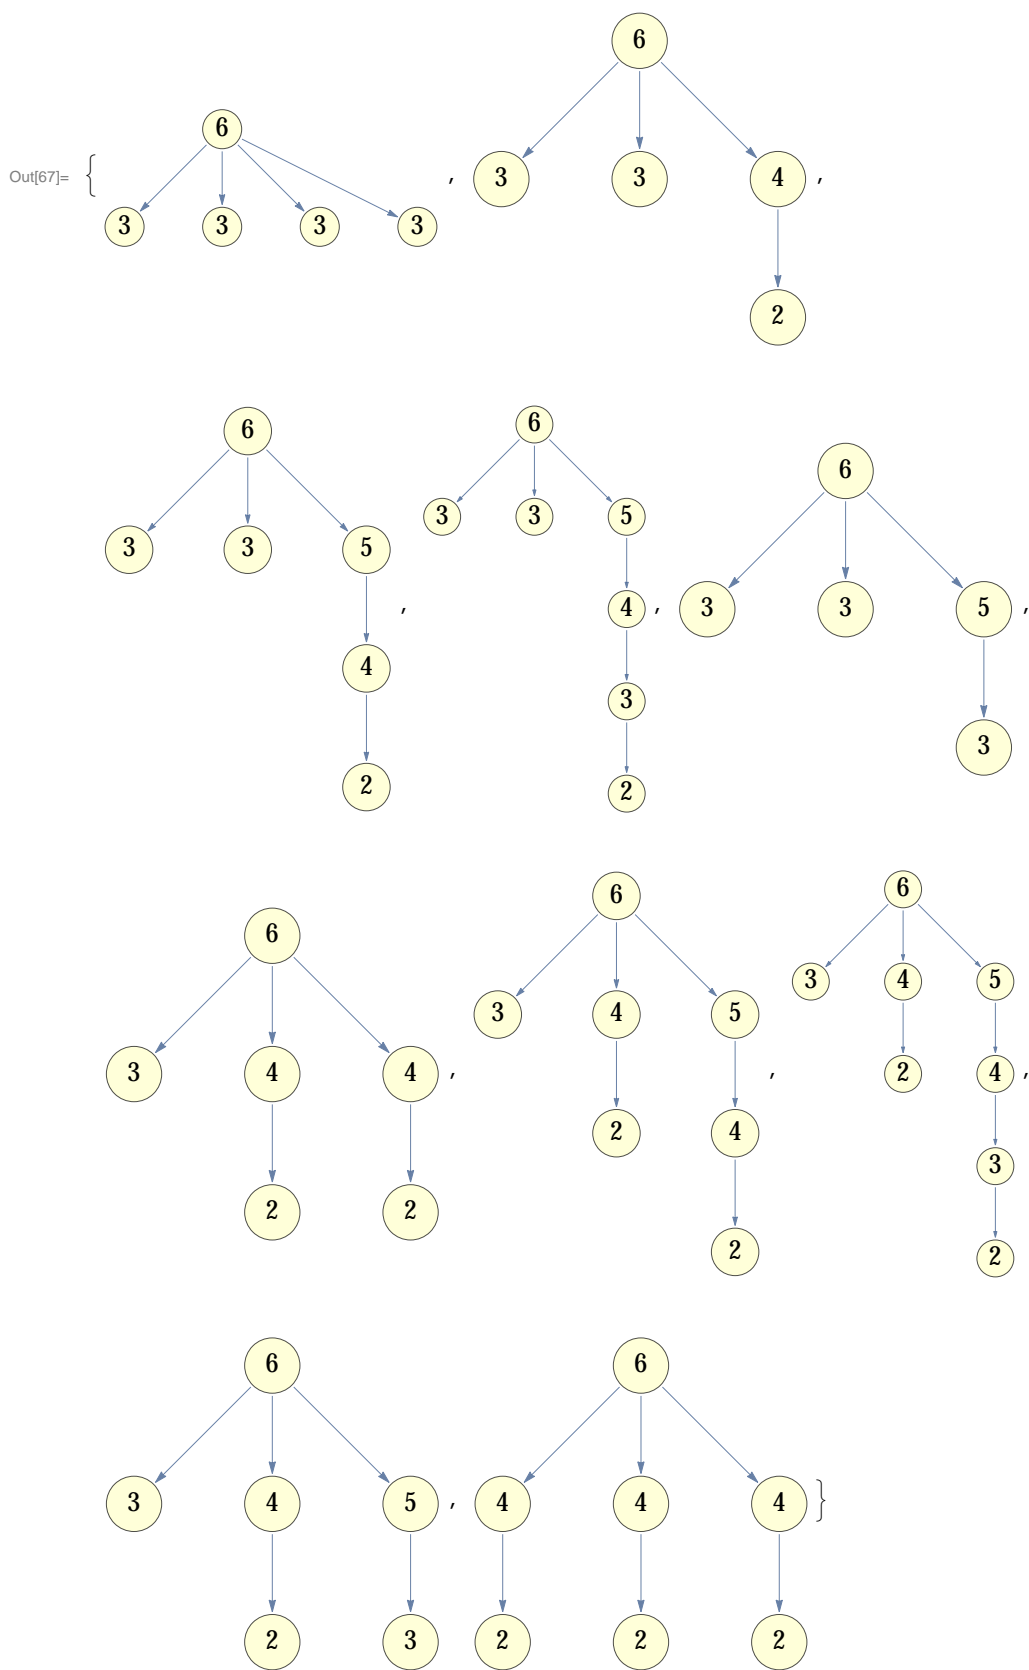

To check that all are Dynkin diagrams, you can do

```
In[68]:= Select[ShowQuiver /@ RemoveVeryObvious[branches[SU[6], 12, bifunds]], NonDynkinQ]
```

```
Out[68]= {}
```

If you're just interested in the top level structure, you can also try

```
In[69]:= ShowQuiver /@ RemoveVeryObvious[branches[SU[6], 12, bifunds, LevelOneOnly -> True]]
```

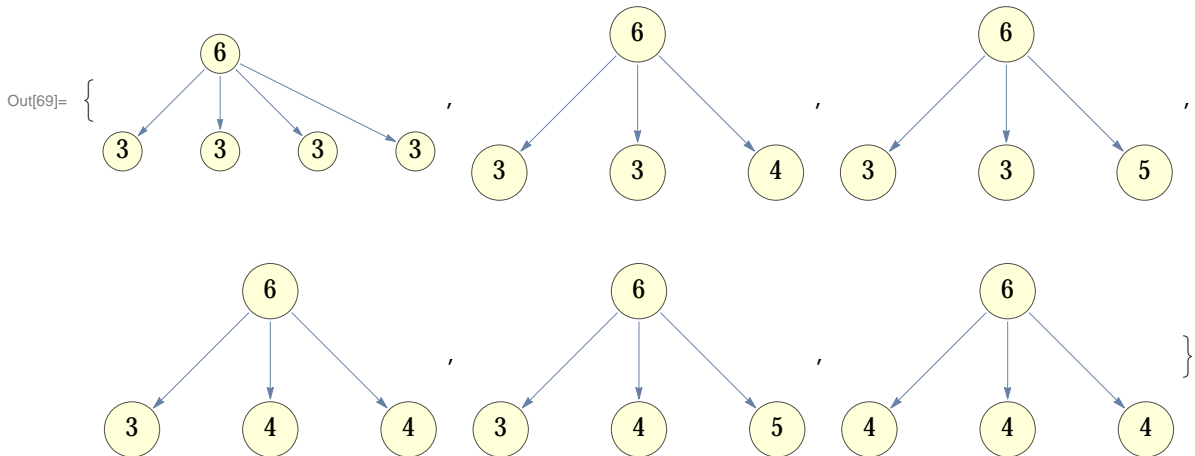

Hopefully you got the idea. Some illustrative examples are:

All the small branches of  $\text{USp}[6]$ .

```
In[70]:= ShowQuiver /@
  branches[USp[6], hvee[USp[6]], Join[bifunds, rarebifunds, idents, matters]]
```

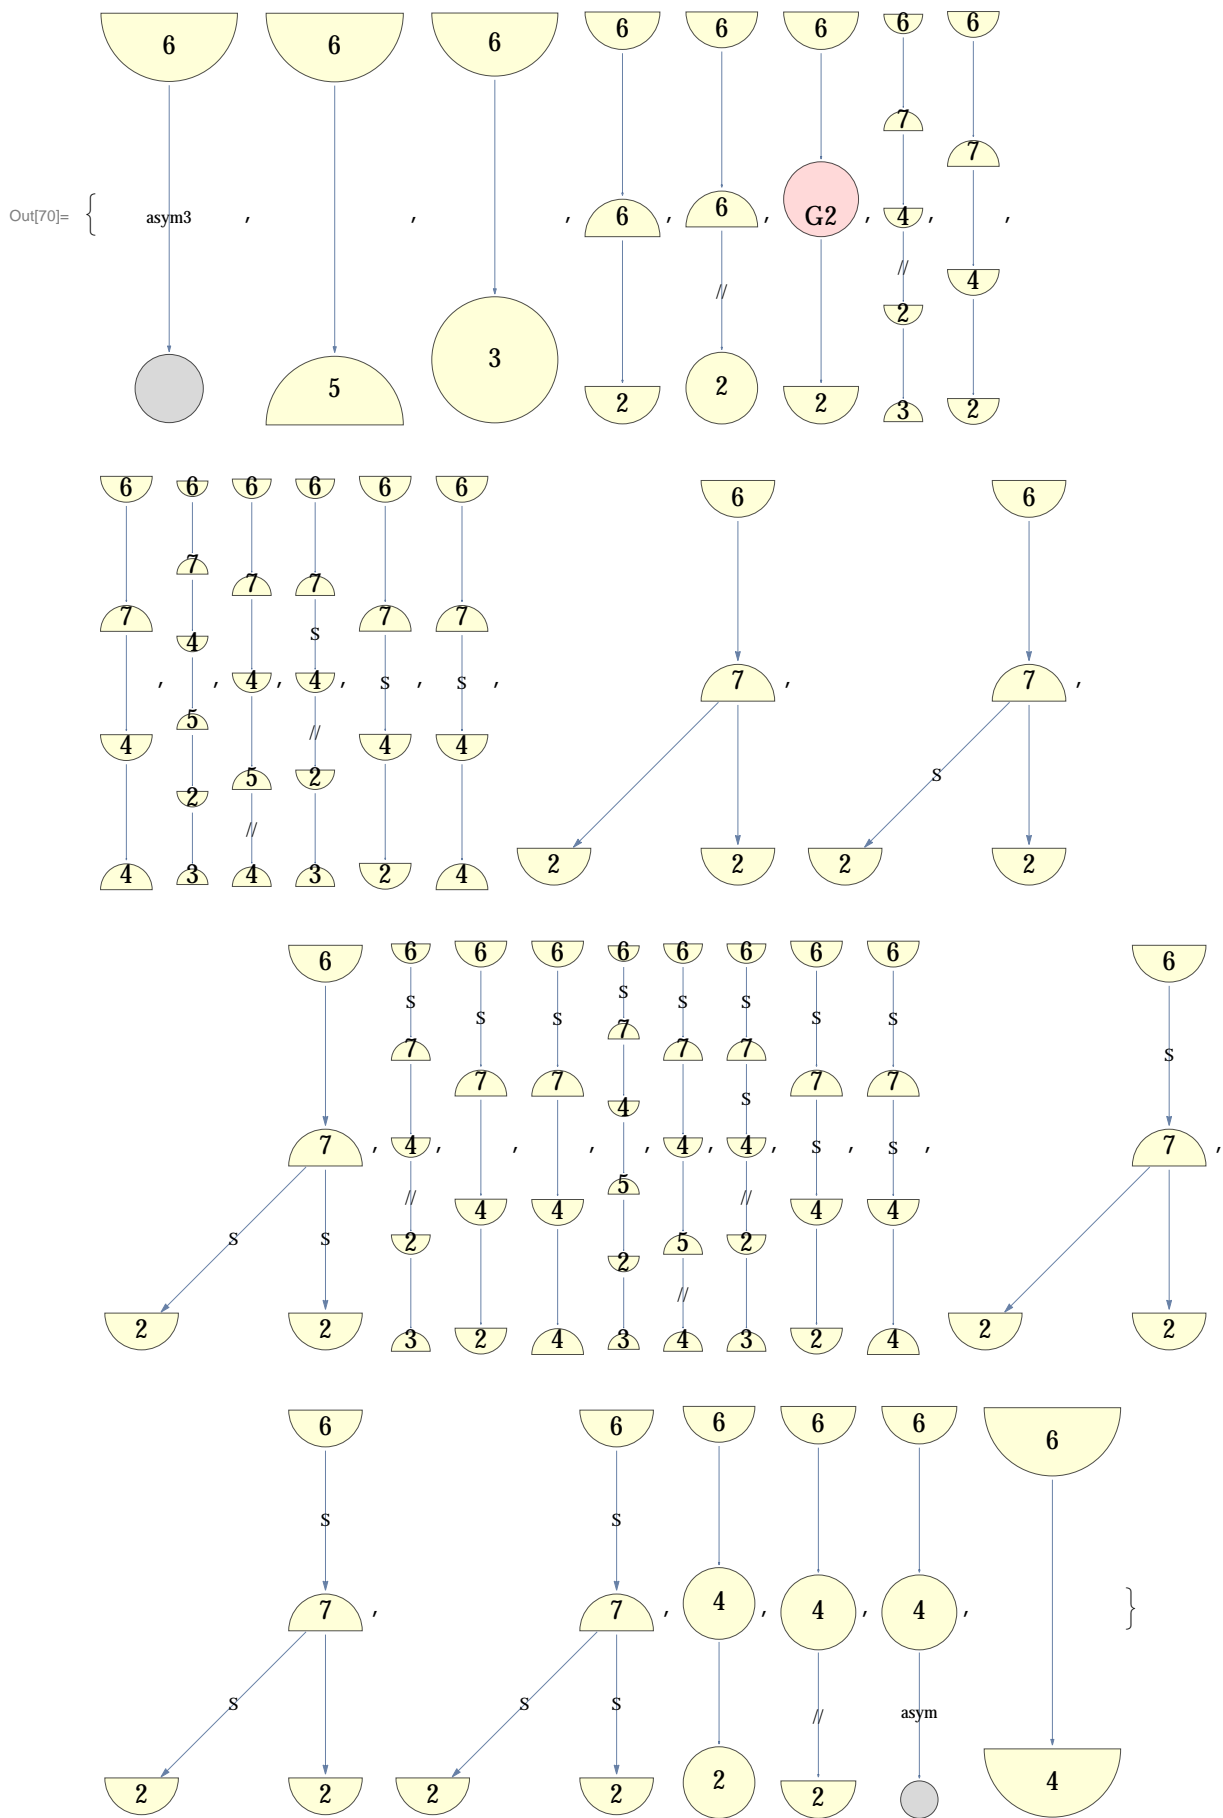

## All “non-Dynkin” theories with a single SO[8] as the trunk using just SO-USp bifundamentals:

```
In[71]:= Select[ShowQuiver /@ branches[SO[8], 2 hvee[SO[8]], bifunds], NonDynkinQ]
```

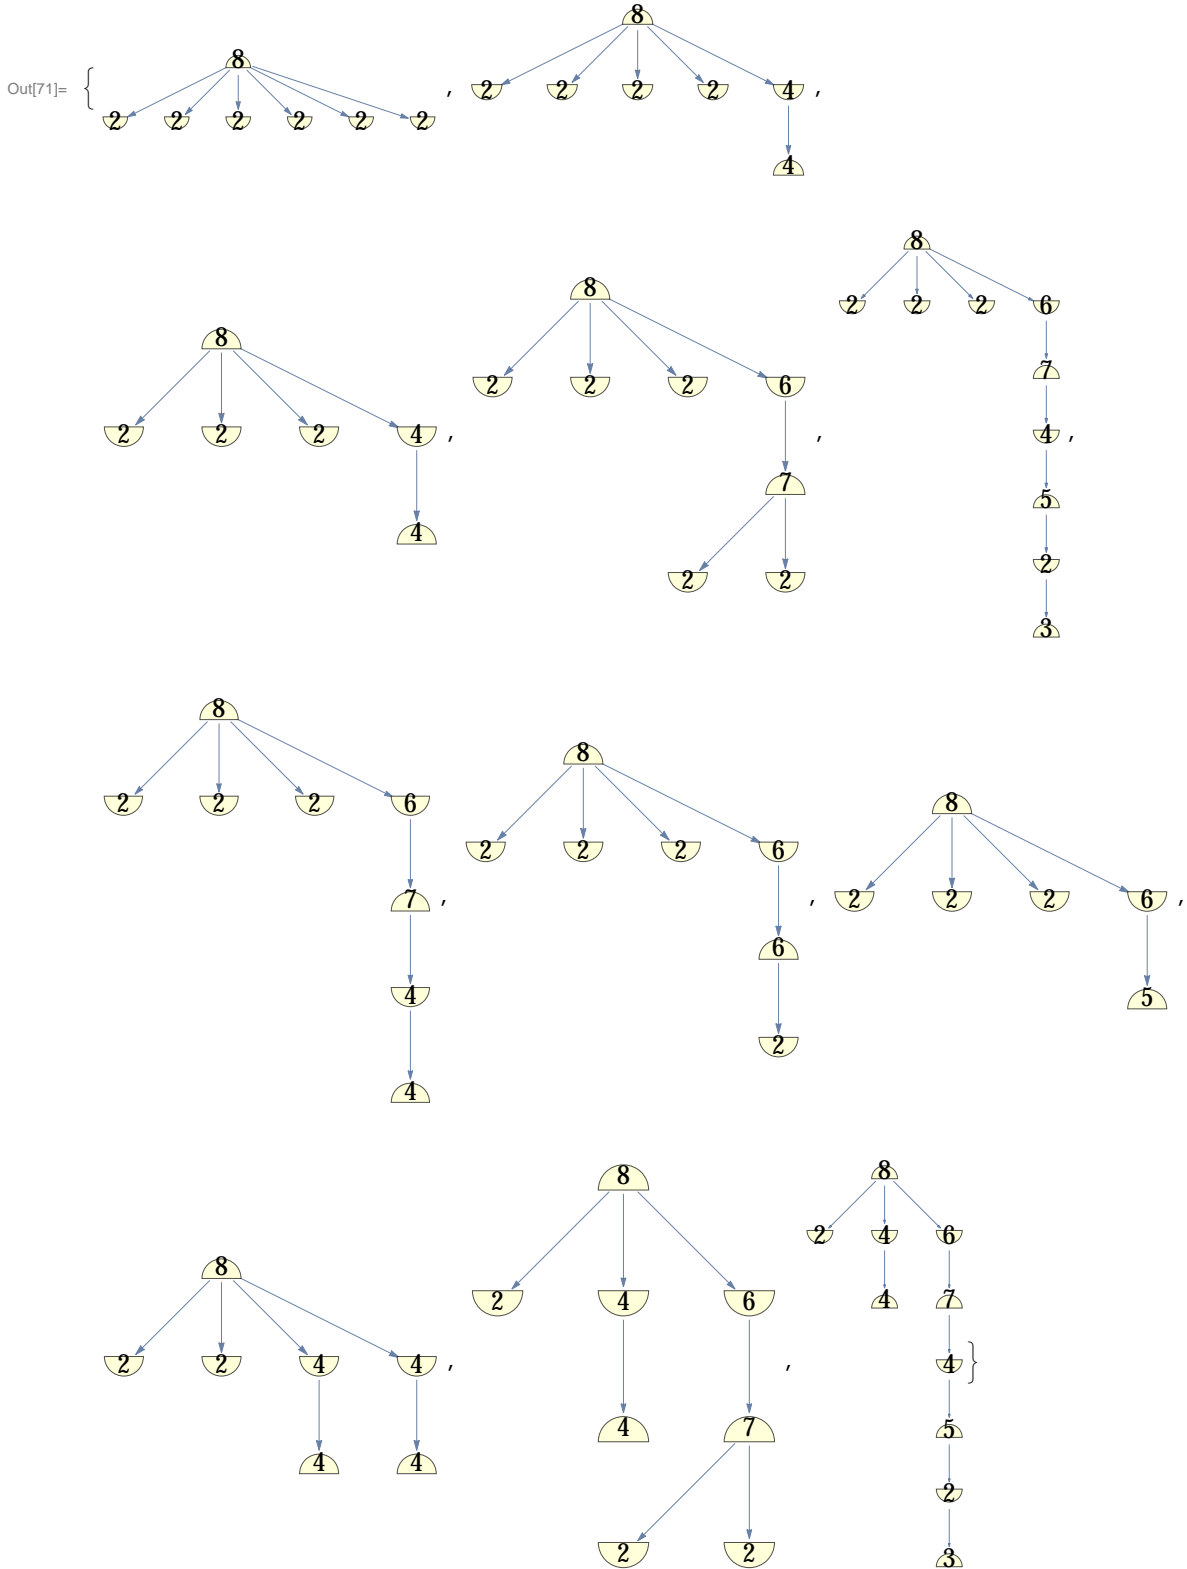

Finally, this lists all theories with a single  $SU(4)$  as the trunk:

```
In[72]:= ShowQuiver /@  
         branches[SU[4], 2 hvee[SU[4]], Join[bifunds, rarebifunds, idents, matters]]
```
